# Supplementary material for: Unsupervised Speech Recognition via Segmental Empirical Output Distribution Matching
Source: arXiv:1812.09323 source file (2018-12-23)
Supplement: Supplementary file 1 [file appendix.tex]

\clearpage
% \section{Appendix}
\appendix
\section{Appendix}
